# Supplementary material for: Pressure induced ferromagnetic to antiferromagnetic phase transition in transition metal chalcogenide Cr$_{3}$Te$_4$
Source: arXiv:2507.07650 ancillary file (2025-07-10)
Supplement: Supplementary file 1 [file supplementary.pdf]

# Supplementary: Pressure induced ferromagnetic to antiferromagnetic phase transition in transition metal chalcogenide $Cr_3Te_4$

Asish Kumar Mishra,[1,2] Souvick Chakraborty,[1] Bidisha Mukherjee,[1,2] Mrinmay Sahu,[1,2] Suvashree Mukherjee,[1,2] Shubham Purwar,[3] Harekrishna Bhunia,[1] S. Thirupathaiah,[3] Peter Liermann,[4] Satyabrata Raj,[1,2] and Goutam Dev Mukherjee[1,2,*]

[1]*Department of Physical Sciences, Indian Institute of Science Education and Research Kolkata, Mohanpur Campus, Mohanpur 741246, Nadia, West Bengal, India.*

[2]*National Centre for High-Pressure Studies, Department of Physical Sciences, Indian Institute of Science Education and Research Kolkata, Mohanpur Campus, Mohanpur 741246, Nadia, West Bengal, India.*

[3]*Department of Condensed Matter and Materials Physics, S. N. Bose National Centre for Basic Sciences, Kolkata, West Bengal 700106, India*

[4]*Photon Science, Deutsches Elektronen Synchrotron, 22607 Hamburg, Germany*

(Dated: July 9, 2025)

[*] Corresponding author: goutamdev@iiserkol.ac.in

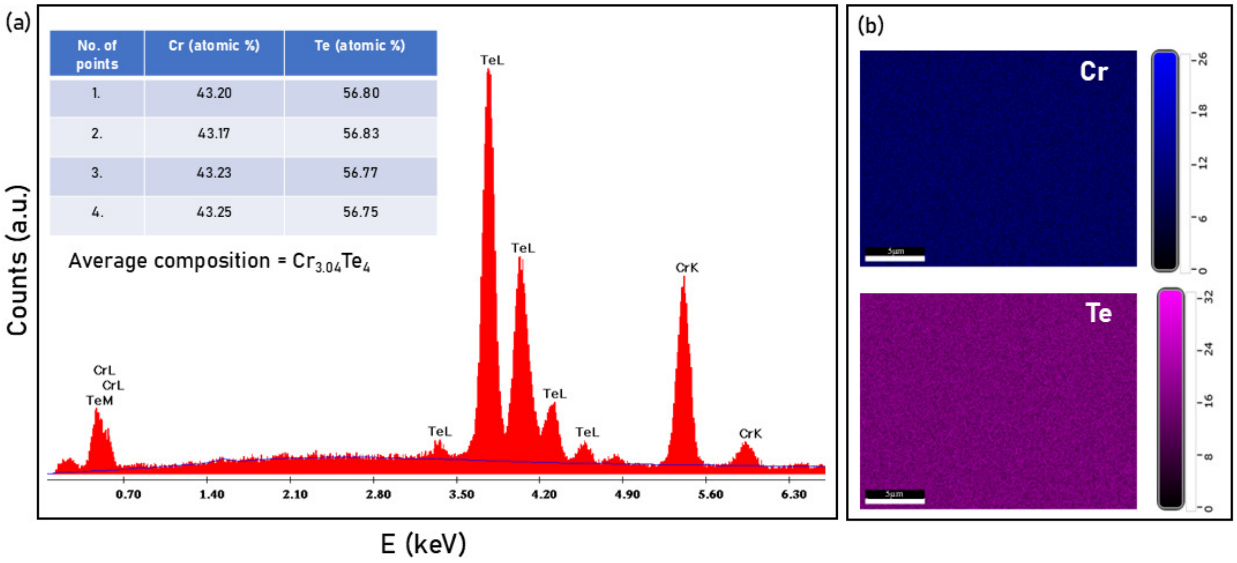


FIG. S1: (a) Shows EDXS data demonstrating the actual chemical composition of the as-grown single crystal. Inset in (a) shows the atomic % of the elemental constituents present in the crystal. (b) Elemental mapping of Cr3Te4 for Cr and Te using EDXS, demonstrating the chemical homogeneity of the studied crystal.

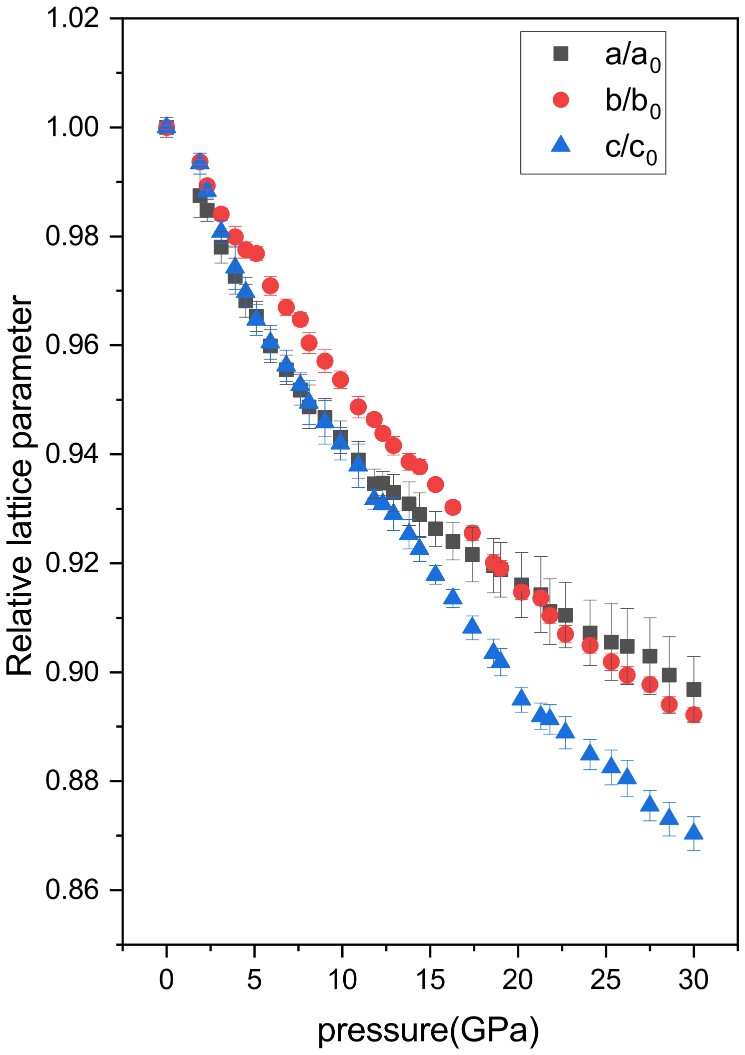


FIG. S2: Relative lattice parameter vs pressure. The black square represents $a/a_0$, red dot shows $b/b_0$ and the blue triangle represents $c/c_0$

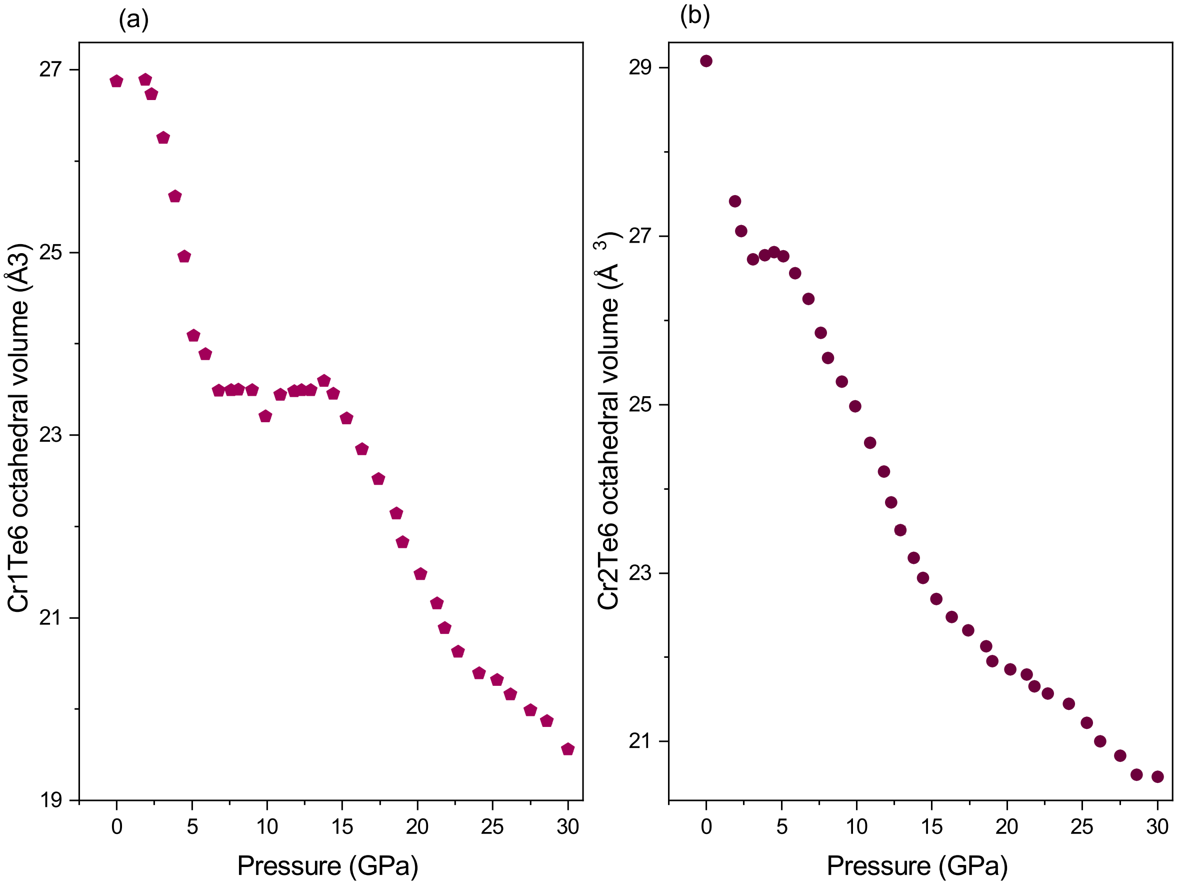


FIG. S3: (a) Cr1-Te6 octahedral volume (b) Cr2-Te6 octahedral volume

(a) (b)

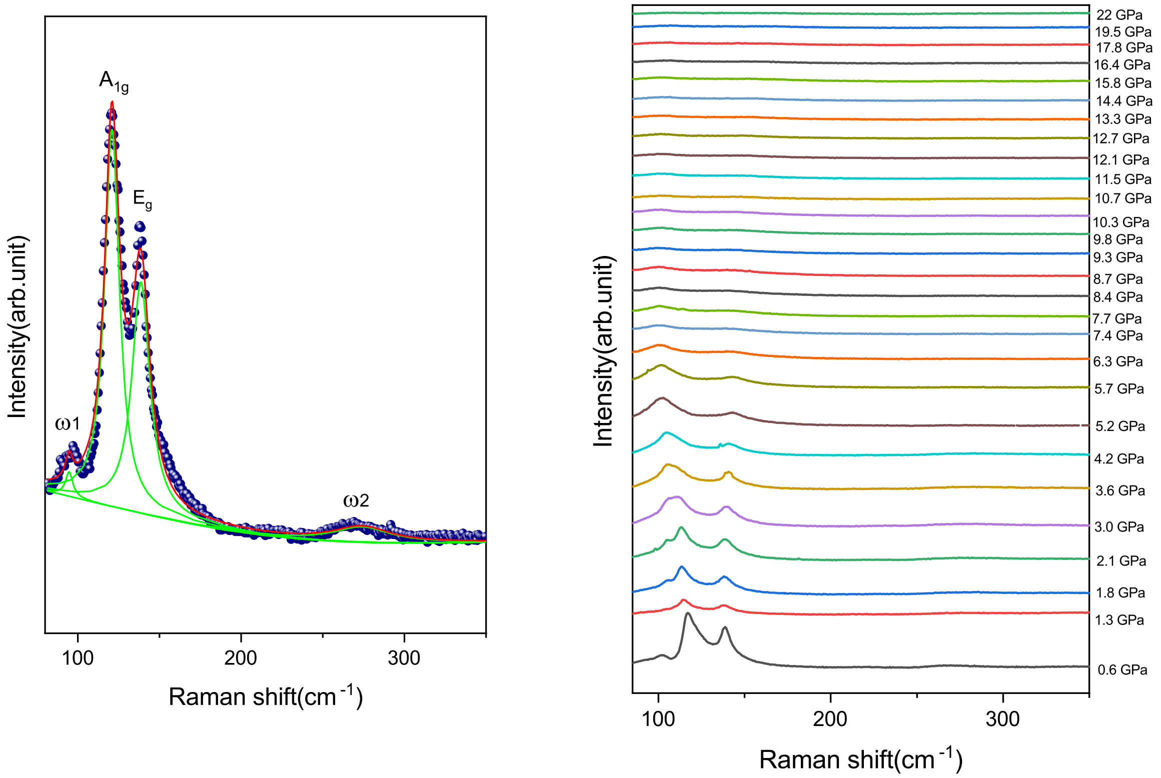


FIG. S4: (a) The Raman spectra at ambient pressure and room temperature. The lorentzian profile is used to fit the background corrected spectrum.(b) Evolution of Raman spectra at all pressure values

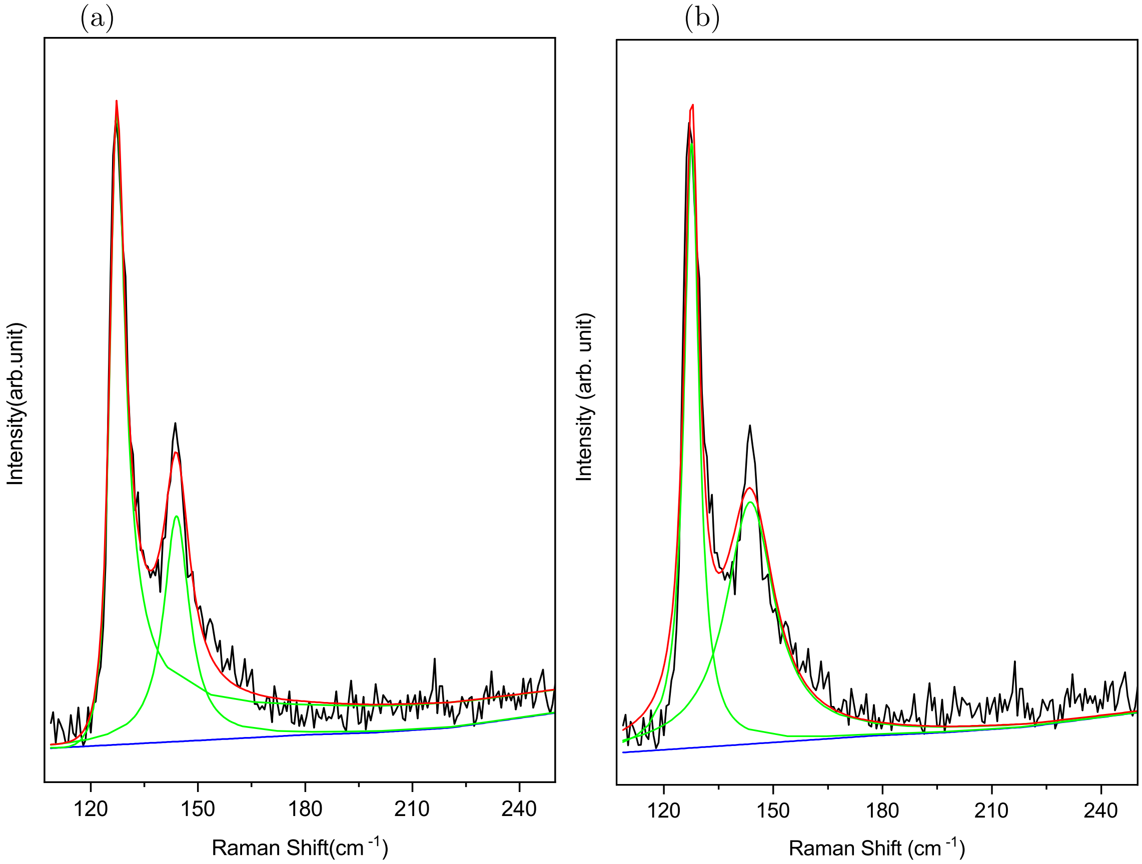


FIG. S5: The Raman spectra at 22K temperature,The red lines are best fit to the experimental data,black lines are the observed experimental data,green lines are the fitting to individual peak and the blue line indicates the background fitting (a) Fitted with BWF and Lorentzian profile (b) Fitted with Lorentzian profile
